# Supplementary material for: BungeeNeRF: Progressive Neural Radiance Field for Extreme Multi-scale Scene Rendering
Source: arXiv:2112.05504 source file (2023-05-09)
Supplement: Supplementary file 1 [file supplementary.tex]

\label{sec:supp}
\newpage

The fidelity of NeRF depends critically on the use of positional encoding, as it allows the MLP parameterizing the scene to behave as an interpolation function, where $L$ determines the bandwidth of the interpolation kernel~\cite{tancik2020fourier}.
For the $k$-th component in the log-linear spaced frequencies, the default PE as proposed in~\cite{mildenhall2020nerf} uses a fourier feature mapping from each input dimension to a higher dimensional hypersphere with $\gamma_{k}(x)=\sin (k x)$\footnote{We eliminate $\gamma_{k}(x) = \cos (kx)$ here for notation brevity.}.

Instead of performing point-sampling along each ray, MipNeRF~\cite{barron2021mip} divide the cone being cast into a series of conical frustum, and constructs an \textbf{integrated positional encoding (IPE)} representation of the volume covered by each conical frustum. They further approximate the conical frustum with a multivariate Gaussian which allows for
an efficient approximation to the desired feature, resulting the IPE as
$E_{x \sim \mathcal{N}\left(\mu, \sigma^{2}\right)}\left[\gamma_{k}(x)\right]=\sin (k \mu) \exp \left(-(k \sigma)^{2} / 2\right).$
These changes allow the MLP to reason about the size and shape of each conical frustum, instead of just its centroid.
Note that IPE could be viewed as a special case of a general \textbf{weighted position encoding}, which assigns a smaller weight to high-frequency components conditioned on the input cone volumns to regularize different frequency bands,
\begin{equation}
	\begin{gathered}
		\gamma_{k}(x)= w_{k}(\alpha) \sin (kx) \\ 
		\text { with } \quad w_{k}(\alpha) = \exp \left(-(k \sigma)^{2} / 2\right)
	\end{gathered}
\end{equation}
Note that \textbf{windowed position encoding} as taken by ~\cite{park2021nerfies, park2020deformable, lin2021barf} also follows this weighted form with
$
w_{k}(\alpha)=\frac{1}{2}(1-\cos (\pi \operatorname{clamp}(\alpha-k, 0,1)))
$ being proportional to the optimization progress.
